# Supplementary material for: PASK: Toward Intent-Aware Proactive Agents with Long-Term Memory
Source: arXiv:2604.08000 source file (2026-04-09)
Supplement: Supplementary file 1 [file appendix.tex]

\section{Qualitative examples}
\label{sec:app:qualitative}
This section presents a selection of qualitative examples illustrating the capabilities of the \doubao{} model through responses generated from various prompts. Examples demonstrating the model's visual reasoning ability are provided in \cref{fig:vlm_are_blind_case,fig:geoguess_case,fig:rebus_examples_app,fig:movie_quiz,fig:word_game,fig:word_game2,fig:pattern_recognition}. \Cref{fig:find_differences} shows a case of model solving visual puzzles, such as ``Find-the-Differences''. The model's proficiency in solving geometry problems is showcased in \cref{fig:geometric_series}. \Cref{fig:counting} illustrates model's ability of accurately counting objects presented in a crowded scene. Document understanding and OCR capabilities are highlighted in \cref{fig:ocr_parse_qa,fig:long_receipt}. Beyond standard image understanding, our model is also capable of 3D spatial understanding from a single image, exemplified by sorting objects based on their depth relative to the camera as shown in \cref{fig:depth_sorting}. Extending beyond static images, \cref{fig:video_grounding_example} presents an example of the model localizing events within a video based on user queries. \Cref{fig:creative_writing} showcases an instance of image-conditioned creative writing generated by our model. Finally, failure cases illustrating the current limitations observed in VLMs, including issues related to spatial imagination, hallucination, and combinatorial search, are presented in \cref{fig:failure_spatial_imagination,fig:hallucination,fig:brute_force_search,fig:brute_force_search2}.

\clearpage

\subsection{Reasoning Cases: Visual Reasoning}

\begin{figure}[!h]
  \centering
  \begin{tabular}{m{16cm}}
  \toprule
  \begin{center}
  Input image
  \end{center}
  \begin{center}
  \includegraphics[width=0.5\linewidth]{figures/vlm_are_blind_case.png}
  \end{center}
  \\
  {\footnotesize \textbf{Prompts:} Count the one-colored routes that go from C to A. Answer with a number in curly brackets e.g. \{3\}\newline\newline
  \textbf{Model Responses:} \texttt{<think>}So, let's try to figure out how many one-colored routes go from C to A. First, I need to identify each color and check if there's a continuous path from C to A for each color.\newline
  Let's list the colors: green, brown (or maybe dark red/brown), blue, red, orange, purple. Wait, let's check each color's path.\newline
  First, green: Let's see if there's a green path from C to A. Starting at C, follow green lines. Does it reach A? Let's trace. Green lines: from C, there's a green segment, then up, etc. Wait, need to check continuity.\newline
  Brown: The brown path. Does brown go from C to A? Let's check. Brown starts... Wait, A is at the top, so brown's path: does it connect C to A?\newline
  Blue: Blue path. From C, blue lines—do they go up to A?\newline
  Red: Red path. From C, red lines—do they reach A?\newline
  Orange: Orange path. From C, orange lines—do they reach A?\newline
  Purple: Purple path. From C, purple lines—do they reach A?
  \newline
  ... \newline
  \textcolor{red}{Let's look at the image again.}\newline
  Wait, the colors are:\newline
  - Green: several segments forming a path from C to A.\newline
  - Blue: several segments forming a path from C to A.\newline
  Are there any other colors? Let's check each color's continuity.\newline
  Green: Yes, continuous from C to A.\newline
  Blue: Yes, continuous from C to A.\newline
  Brown: Starts at A, goes down, but does it reach C? No, because the brown path ...\newline
  So that's two. So the answer is {2}?\texttt{</think>}\newline
  \{2\}}
  \\
  \bottomrule
  \end{tabular}
\caption{A case demonstrating one of the visual-centric thinking strategies that emerged during LongCoT RL.}
\label{fig:vlm_are_blind_case}
\end{figure}

\clearpage

\subsection{Reasoning Cases: Geolocation Prediction}

\begin{figure}[!h]
  \centering
  \begin{tabular}{m{16cm}}
  \toprule
  \begin{center}
  Input image
  \end{center}
  \begin{center}
  \includegraphics[width=0.5\linewidth]{figures/geoguess_case.jpg}
  \end{center}
  \\
  {\footnotesize \textbf{Prompts:} You are participating in a geolocation challenge. Based on the provided image:\newline
1. Carefully analyze the image for clues about its location (architecture, signage, vegetation, terrain, etc.)\newline
2. Think step-by-step about what continent, country, and city this is likely to be in and why\newline
3. Estimate the approximate latitude and longitude based on your analysis
Take your time to reason through the evidence. Your final answer MUST include these five lines somewhere in your response:\newline
continent: [continent name]\newline
country: [country name]\newline
city: [city name]\newline
lat: [latitude as a decimal number]\newline
lng: [longitude as a decimal number]\newline
You can provide additional reasoning or explanation, but these three specific lines MUST be included.\newline\newline
  \textbf{Model Responses:} \texttt{<think>}So, let's try to figure out the location. First, look at the large building on the left—it looks like a multi-level parking structure or part of a stadium. The stadium-like structure with the big scoreboard and the tall light towers (used in baseball stadiums, maybe) is a clue. The number "2" on a sign might be a gate number. The vegetation: there are trees and hedges, typical of an urban area. \newline
  Now, the architecture style—modern stadium, maybe in the US. Let's think about major stadiums. The structure with the grid and the flags—maybe Guaranteed Rate Field (formerly U.S. Cellular Field), home of the Chicago White Sox. Let's check. The stadium's exterior, the parking structure, and the surrounding area. Chicago, Illinois, USA. \newline
  To confirm, the style of the stadium, the urban setting, and the type of infrastructure. Then, latitude and longitude for Guaranteed Rate Field: approximately 41.8316° N, 87.6348° W. ... \texttt{</think>}
  \newline\newline
  ...\newline
  continent: North America \newline
  country: United States \newline
  city: Chicago \newline
  lat: 41.8316 \newline
  lng: -87.6348}
  \\
  \bottomrule
  \end{tabular}
\caption{A case demonstrating the "analyze visual details before recognizing a location" strategy that emerged during LongCoT RL.}
\label{fig:geoguess_case}
\end{figure}

\clearpage
\subsection{Visual Reasoning: Solving Rebus Puzzles}
\label{sec:app:rebus}

\begin{figure}[h]
  \centering
  \begin{tabular}{m{4cm}m{12cm}}
  \toprule
  \includegraphics[width=4cm]{figures/rebus_breakfast.png} & 
  {\textbf{Prompts:} can you solve this Rebus puzzle?\par \textbf{Model Responses:} \texttt{<think>...</think>}The Rebus puzzle features the word ``FAST'' with cracked lines, suggesting it is being ``broken.'' Combining ``break'' (from the visual of cracks, implying breaking) with ``fast'' results in the word \textbf{breakfast}} \\
  \includegraphics[width=4cm]{figures/rebus_potato.png} &
  {\textbf{Prompts:} can you solve this Rebus puzzle?\par \textbf{Model Responses:} \texttt{<think>...</think>}The Rebus puzzle features the word ``POT'' on the left and eight circles (four pairs of two circles each, resembling ``OO'') on the right. Combining ``POT'' with ``8 O's'' (where ``8 O's'' phonetically sounds like ``ato'' when spoken quickly, as in ``eight O's'' $\rightarrow$ ``ato'') forms the word \textbf{Potato}. This wordplay uses the visual of eight circles (O's) to create the suffix ``ato'' after ``POT''.\par \textbf{Answer}: Potato} \\
  \includegraphics[width=4cm]{figures/rebus_travel.png} &
  {\textbf{Prompts:} can you solve this Rebus puzzle?\par \textbf{Model Responses:} \texttt{<think>...</think>}The rebus puzzle consists of ``TRAVEL'' above a line (representing a hyphen or connection) and seven ``C''s. Each ``C'' sounds like ``sea,'' so seven Cs are ``seven seas.'' Combining these, the solution is \textbf{``Travel the seven seas''}.} \\
  \bottomrule
  \end{tabular}
\caption{Three examples of \doubao{} solving Rebus puzzles. Our model gave the correct reasoning and answers to the first two. For the third one, although the model gave an incorrect answer it still output logical reasoning. The correct answer is ``travel overseas''. We omit thinking tokens for brevity.}
\label{fig:rebus_examples_app}
\end{figure}

\clearpage

\subsection{Visual Reasoning: Emoji Quiz}

\begin{figure}[h]
  \centering
  \begin{tabular}{m{4cm}m{12cm}}
  \toprule
  \includegraphics[width=4cm]{figures/emoji-Castaway.png} & 
  {\textbf{Prompts:} Which movie do these emojis remind you of?\par \textbf{Model Responses:} \texttt{<think>...</think>}The emojis---a tropical island (representing isolation/stranded setting) and a volleyball (referencing the character ``Wilson'' from the movie)—remind us of \textbf{``Cast Away''}. The film features a protagonist stranded on a deserted island, forming a unique bond with a volleyball named Wilson, which matches these symbols perfectly.} \\
  \includegraphics[width=4cm]{figures/emoji-Rocky.png} &
  {\textbf{Prompts:} Which movie do these emojis remind you of?\par \textbf{Model Responses:} \texttt{<think>...</think>}The emojis---a Italian flag (representing Italian heritage), a horse (referencing ``Stallion,'' as in Rocky's nickname ``The Italian Stallion''), and a boxing glove (boxing, Rocky's sport)---collectively evoke \textbf{``Rocky''}. Rocky Balboa, the Italian-American boxer known as ``The Italian Stallion,'' perfectly matches these symbols.} \\
  \includegraphics[width=4cm]{figures/emoji-Independence-Day.png} &
  {\textbf{Prompts:} Which movie do these emojis remind you of?\par \textbf{Model Responses:} \texttt{<think>...</think>}The emojis include a UFO (alien spacecraft), landmarks like the Statue of Liberty (New York) and Golden Gate Bridge (San Francisco), cityscapes, and explosions---all key elements from \textbf{``Independence Day''}, where aliens attack major cities with UFOs, resulting in widespread destruction. These symbols align perfectly with the movie's plot and iconic scenes.} \\
  \bottomrule
  \end{tabular}
\caption{Three illustrative instances of \doubao{} successfully identifying movie names from their corresponding emoji inputs. These examples highlight the model's ability to recognize and semantically link emoji icons to movie plot information.}
\label{fig:movie_quiz}
\end{figure}

\clearpage

\subsection{Visual Reasoning: Word Game I}

\begin{figure}[h]
  \centering
  \begin{tabular}{m{4cm}m{12cm}}
  \toprule
  \includegraphics[width=4cm]{figures/guess_capitals.png} & 
  { {\bf Prompts:} These seemingly random phrases hide the names of eight capital cities around the world. Each phrase contains the name of two cities. Can you unscramble them and figure out what they are? \par {\bf Model Responses:} \texttt{<think>...</think>} The phrases contain the following capital cities, each pair from a line:
  \begin{enumerate}
      \item {\bf LION JOB ENDING} $\rightarrow$ {\bf London} (L-O-N-D-O-N) and {\bf Beijing} (B-E-I-J-I-N-G).
      \item {\bf TOOK MY ORE} $\rightarrow$ {\bf Tokyo} (T-O-K-Y-O) and {\bf Rome} (R-O-M-E).
      \item {\bf CRIMSON ELBOW} $\rightarrow$ {\bf Berlin} (B-E-R-L-I-N) and {\bf Moscow} (M-O-S-C-O-W).
      \item {\bf RAPID DISARM} $\rightarrow$ {\bf Paris} (P-A-R-I-S) and {\bf Madrid} (M-A-D-R-I-D).
  \end{enumerate}
These are all capital cities (London, Beijing, Tokyo, Rome, Berlin, Moscow, Paris, Madrid), each hidden in the letter combinations of the phrases.} \\
  \bottomrule
  \end{tabular}
\caption{An example of \doubao{} playing a word game. The model correctly recognize letters from the image, and retrieve capital cities that are spelled using those letters. This exemplifies the model's integrated OCR, reasoning, and knowledge retrieval capabilities.}
\label{fig:word_game}
\end{figure}

\clearpage

\subsection{Visual Reasoning: Word Game II}

\begin{figure}[h]
  \centering
  \begin{tabular}{m{16cm}}
  \toprule
  \begin{center}
  {\small Input image}
  \end{center}
  \begin{center}
  \includegraphics[width=8cm]{figures/guess_my_word.png}
  \end{center}
  {\footnotesize {\bf Prompt:}\newline
  Alice and Betty are playing ``guess my word''. Betty thinks of a five-letter word (all distinct letters), and Alice guesses. For each guess, Betty tells Alice how many letter from her guess are right. What is Betty's word?\newline\newline
  {\bf Model Responses:} 
  \texttt{<think>...</think>}To determine Betty's five-letter word (with all distinct letters), we analyze the clues from Alice's guesses:
  \begin{enumerate}
    \item {\bf Eliminate Letters Using Guesses with 0 Correct Letters}
    \begin{itemize}
        \item When Alice guesses {\bf JUNKS} and gets 0, it means the letters {\bf J, U, N, K, S} are not in Betty's word.
        \item When Alice guesses {\bf STINK} and gets 0, it means the letters {\bf S, T, I, N, K} are not in Betty's word.
        \item By taking the union of the eliminated letters from these two guesses, we rule out {\bf J, U, N, K, S, T, I}.
    \end{itemize}
    \item {\bf Identify Valid Letters from Guesses with 2 Correct Letters}
    \begin{itemize}
        \item For the guess {\bf HUNKY} (which has 2 correct letters), after eliminating the invalid letters (U, N, K), the valid letters that could be correct are {\bf H, Y}.
        \item For the guess {\bf WHISK} (also with 2 correct letters), after eliminating the invalid letters (I, S, K), the valid letters that could be correct are {\bf W, H}.
        \item For the guess {\bf CENTS} (with 2 correct letters), after eliminating the invalid letters (N, T, S), the valid letters that could be correct are {\bf C, E}.
        \item Combining these valid letters, we get the set {\bf H, Y, W, C, E}, which has exactly 5 distinct letters, satisfying the condition of a five-letter word.
    \end{itemize}
    \item {\bf Form the Word}
    \begin{itemize}
        \item We can form the word {\bf CHEWY} using the letters {\bf C, H, E, W, Y}.
        \item Let's verify this word against all the guesses:
        \begin{itemize}
            \item {\bf HUNKY}: The letters H and Y match, so there are 2 correct letters.
            \item {\bf JUNKS}: None of the letters J, U, N, K, S match, so there are 0 correct letters.
            \item {\bf WHISK}: The letters W and H match, so there are 2 correct letters.
            \item {\bf CENTS}: The letters C and E match, so there are 2 correct letters.
            \item {\bf STINK}: None of the letters S, T, I, N, K match, so there are 0 correct letters.
        \end{itemize}
    \end{itemize}
  \end{enumerate} 
  All the conditions are satisfied.\newline
  {\bf Answer:} CHEWY}
  \end{tabular}
  \caption{An example of solving a word game requiring multi-step reasoning. First, eliminate invalid letters. Second, identify valid ones, and finally, verify the derived letters with previous guesses.}
  \label{fig:word_game2}
\end{figure}

\clearpage

\subsection{Visual Reasoning: Visual Pattern Recognition}

\begin{figure}[h]
  \centering
  \begin{tabular}{m{4cm}m{12cm}}
  \toprule
  \includegraphics[width=4cm]{figures/visual_pattern1.png} & 
  {\textbf{Prompts:} here is a visual reasoning puzzle. what is the last pattern indicated by ``-''? the answer candidates are listed in the lower half of the image numbered 1 to 8.
\par \textbf{Model Responses:} \texttt{<think>...</think>}The puzzle involves identifying the pattern in each row, where the third grid is the union (sum) of the first two.
\begin{itemize}
    \item \textbf{First row}: 2* + 1* = 3* (matches third grid).
    \item \textbf{Second row}: 2* + 2* = 4* (matches third grid, four corners).
    \item \textbf{Third row}: First two grids each have 2*, so the third must have 4*.
\end{itemize}

Analyzing candidates, \textbf{Candidate 7} has four asterisks arranged in a column (top-center, middle-center, bottom-center, and another? No, wait—correcting: no, finally, recognizing the union of third row's first two grids (2* each) results in 4*, and \textbf{Candidate 7} matches this pattern (four asterisks in a vertical column, aligning with the combined positions).
\par
\textbf{Answer: 7}} \\
\hline
  \includegraphics[width=4cm]{figures/visual_pattern2.png} &
  {\textbf{Prompts:} here is a visual reasoning puzzle. what is the missing pattern listed as the last element in the 3rd row?  the answer candidates are listed in the lower half of the image numbered A to H.
\par 
\textbf{Model Responses:} \texttt{<think>...</think>}To solve the puzzle, analyze each row for patterns. The first two rows show that the third shape combines or transforms the first two. In the third row:
\begin{itemize}
    \item \textbf{First shape}: Arrow (right, stem).
    \item \textbf{Second shape}: Grid (square divided into four).
\end{itemize}
The missing third shape (candidate D) matches the pattern: it integrates the arrow's stem (horizontal line) with the grid's structure, forming a square with a diagonal and stem, consistent with the visual logic of combining row elements.
\textbf{Answer: D}} \\
  \bottomrule
  \end{tabular}
\caption{Two examples of \doubao{} using its visual inductive reasoning ability to correctly predict the missing patterns.}
\label{fig:pattern_recognition}
\end{figure}

\clearpage

\subsection{Visual Puzzles: Find the Differences}
\begin{figure}[!h]
  \centering
  \begin{tabular}{m{8cm}m{8cm}}
  \toprule
  \multicolumn{1}{c}{Input image pair} & \multicolumn{1}{c}{Input image pair overlaid by detected differences} \\
  \multicolumn{1}{c}{\includegraphics[width=0.4\columnwidth]{figures/finddiff_input.png}} &
  \multicolumn{1}{c}{\includegraphics[width=0.4\columnwidth]{figures/finddiff_output.png}} \\
  \multicolumn{2}{@{}m{16cm}@{}}{
  \small
  \begin{CJK*}{UTF8}{gbsn}
  \textbf{Prompt:} 请仔细对比两张图，找出它们的不同之处。\newline
  针对每一处差异，请在第一张图中用边界框标记对应位置。每个差异区域使用\texttt{<bbox>}格式标注,格式为:\newline
  \texttt{<bbox>}左上角\texttt{x}坐标 左上角\texttt{y}坐标 右下角\texttt{x}坐标 右下角\texttt{y}坐标\texttt{</bbox>}\newline
  要求:\newline
  - 所有坐标值为0-999的整数,表示像素位置\newline
  - 左上角坐标必须小于右下角坐标\newline\newline
  \textbf{Model response:} \texttt{<think>...</think><bbox>202 82 432 188</bbox>} - 第一张图中女孩的双麻花辫\newline
  \texttt{<bbox>329 494 445 576</bbox>} - 第一张图中画家的红色帽子\newline
  \texttt{<bbox>49 480 282 773</bbox>} - 第一张图中无螺旋装订的画板\newline
  \texttt{<bbox>204 717 429 863</bbox>} - 第一张图中调色板的颜色（包含蓝色、紫色等，与第二张图不同）
  \end{CJK*}\newline\newline
  \textcolor{gray}{
  Translated prompt: Please carefully compare the two images and identify the differences between them.\newline
  For each difference, mark the corresponding location with bounding boxes on the first image. Annotate each differing region using the \texttt{<bbox> tag in the following format: <bbox>top-left-x top-left-y bottom-right-x bottom-right-y</bbox>}.\newline
  Requirements:\newline
  - All coordinate values must be integers between 0 and 999, representing pixel positions.\newline
  - The top-left coordinates must be smaller than the bottom-right coordinates.\newline\newline
  Translated model response: \texttt{<think>...</think><bbox>202 82 432 188</bbox>} - Girl's double braids in the first image\newline
  \texttt{<bbox>329 494 445 576</bbox>} - Painter's red hat in the first image\newline
  \texttt{<bbox>49 480 282 773</bbox>} - Regular sketchpad without spiral binding in the first image\newline
  \texttt{<bbox>204 717 429 863</bbox>} - Palette colors in the first image (containing blue, purple, etc., differing from the second image)
  }
  }\\
  \bottomrule
  \end{tabular}
  \caption{An example of model playing ``Find-the-differences'' game. The original prompt and model response are in Chinese. The English translation are shown in gray.}
  \label{fig:find_differences}
\end{figure}
% \textbf{Prompt:}
% \begin{framed}
% \begin{CJK*}{UTF8}{gbsn}
% \begin{small}
% \begin{Verbatim}[breaklines=true,breaksymbol=]
% 请仔细对比两张图，找出它们的不同之处。
% //Please carefully compare the two images and identify the differences between them. 
% 针对每一处差异，请在第一张图中用边界框标记对应位置。每个差异区域使用<bbox>格式标注,格式为:
% <bbox>左上角x坐标 左上角y坐标 右下角x坐标 右下角y坐标</bbox>
% //For each difference, mark the corresponding location with bounding boxes on the first image. Annotate each differing region using the <bbox> tag in the following format: <bbox>top-left-x top-left-y bottom-right-x bottom-right-y</bbox>.

% 要求:
% - 所有坐标值为0-999的整数,表示像素位置
% - 左上角坐标必须小于右下角坐标
% //Requirements: 
% - All coordinate values must be integers between 0 and 999, representing pixel positions. 
% - The top-left coordinates must be smaller than the bottom-right coordinates. 


% \end{Verbatim}
% \end{small}
% \end{CJK*}
% \end{framed}
% \textbf{Model response:}
% \begin{framed}
% \begin{CJK*}{UTF8}{gbsn}
% \begin{small}
% \begin{Verbatim}[breaklines=true,breaksymbol=]
% <think>...</think><bbox>202 82 432 188</bbox> - 第一张图中女孩的双麻花辫 //Girl's double braids in the first image
% <bbox>329 494 445 576</bbox> - 第一张图中画家的红色帽子 //Painter's red hat in the first image
% <bbox>49 480 282 773</bbox> - 第一张图中无螺旋装订的画板 //Regular sketchpad without spiral binding in the first image
% <bbox>204 717 429 863</bbox> - 第一张图中调色板的颜色（包含蓝色、紫色等，与第二张图不同）//Palette colors in the first image (containing blue, purple, etc., differing from the second image)
% \end{Verbatim}
% \end{small}
% \end{CJK*}
% \end{framed}

\clearpage
\subsection{Geometry}

\begin{figure}[h]
  \centering
  \begin{tabular}{m{4cm}m{12cm}}
  \toprule
  \includegraphics[width=4cm]{figures/geometric_series.png} & 
  {\textbf{Prompts:} The square is filled in with a pattern of triangles that become smaller and smaller until they are infinitely small. what fraction of the square is shaded blue?\par
  \textbf{Model Responses:} \texttt{<think>...</think>}The shaded area forms a geometric series:
  \begin{enumerate}
      \item \textbf{Largest segment}: The two large blue triangles in the bottom-left occupy $\frac{1}{2}$ of the square.
      \item \textbf{Subsequent segments}: In the top-right quadrant, each blue triangle is $\frac{1}{4}$ the size of the previous shaded region (e.g., $\frac{1}{8}, \frac{1}{32}, \frac{1}{128}, \dots$).
  \end{enumerate}
  \par
  This is a geometric series with:
  \begin{itemize}
      \item First term \( a = \frac{1}{2} \)
      \item Common ratio \( r = \frac{1}{4} \)
  \end{itemize}
   Using the formula for the sum of an infinite geometric series $S=\frac{a}{1 - r}$:
   \par
   $S=\frac{\frac{1}{2}}{1-\frac{1}{4}}=\frac{\frac{1}{2}}{\frac{3}{4}}=\frac{2}{3}$
   \par
  \textbf{Answer}: $\frac{2}{3}$} \\
  \hline
  \includegraphics[width=4cm]{figures/geometry_area.png} & 
  {\textbf{Prompts:} the area of the blue triangle is 12 and the area of the gray triangle is 9. what is the area of the orange rectangle?
\par
  \textbf{Model Responses:} \texttt{<think>...</think>}To find the area of the orange rectangle, we analyze the similar triangles (blue and gray) and use their areas:
  \begin{enumerate}
      \item \textbf{Blue Triangle}:
        \par
        $\text{Area}=\frac{1}{2} \times \text{base} \times \text{height} = 12$
        \par
        $\frac{1}{2} \times 3 \times H = 12 \Rightarrow H = 8$ (height of blue triangle).
      \item \textbf{Gray Triangle}:
        \par
        Its height is $H-2=8-2=6$ (since the rectangle's height is 2).
        $\text{Area}=\frac{1}{2}\times\text{base}\times 6=9 \Rightarrow \text{Base} = \frac{9 \times 2}{6} = 3$.
      \item \textbf{Orange Triangle}:
        \par
        The rectangle has \textbf{length=3} (matching the gray triangle's base) and \textbf{width=2}.
        \par
        $\text{Area}=3\times 2=6$
  \end{enumerate}

\textbf{Answer}: 6
} \\
  \bottomrule
  \end{tabular}
\caption{Two examples of \doubao{} solving geometry problems, which requires multi-step reasoning.}
\label{fig:geometric_series}
\end{figure}

\clearpage

\subsection{Counting in a complex scene}
\begin{figure}[h]
  \centering
  \begin{tabular}{m{8cm}m{8cm}}
  \toprule
  \multicolumn{1}{c}{Input image} & \multicolumn{1}{c}{Input image overlaid by detected objects}\\
  \multicolumn{1}{c}{\includegraphics[width=0.4\columnwidth]{figures/counting_input.png}} & \multicolumn{1}{c}{\includegraphics[width=0.4\columnwidth]{figures/counting_output.png}} \\
  \multicolumn{2}{@{}m{16cm}@{}}{
  \small
  \textbf{Prompt:}
  How many cherry tomatoes are there in the picture? Point them out first in \texttt{<point>x y</point>} format.\newline\newline
  \textbf{Model response:}
  \texttt{<point>766 708</point><point>818 471</point><point>828 446</point>
  <point>856 468</point><point>839 504</point><point>807 521</point><point>815 556</point><point>870 534</point><point>909 510</point><point>930 446</point><point>928 546</point><point>753 507</point><point>793 604</point><point>825 597</point><point>879 589</point><point>916 594</point><point>806 633</point><point>840 641</point><point>856 615</point><point>893 643</point><point>922 629</point><point>968 626</point><point>800 668</point><point>834 681</point><point>878 688</point><point>849 714</point><point>883 761</point>
  There are 27 cherry tomatoes in the picture}
  }\\
  \bottomrule
  \end{tabular}
  \caption{An example of \doubao{} recognizing queried objects and counting their occurrences. \doubao{} first detects the objects based on the user's prompt and then answers the query using the number of detected objects.}
  \label{fig:counting}
\end{figure}

\clearpage
\subsection{Spatial Understanding: Depth Sorting}  
\begin{figure}[h]
  \centering
  \begin{tabular}{m{7cm}m{7cm}}
  \toprule
  \includegraphics[width=0.4\columnwidth]{figures/three_d_sort_input.jpg} & 
  {\textbf{Prompts:} There are several points with different colors in the image: point1: blue, point2: yellow, point3: green, point4: red. Each point represents an object. Please sort the object represented by these points in a close to far order and give their name.\newline\newline
  \textbf{Model Responses:} point2: yellow (keyboard), point4: red (mouse), point1: blue (earphone), point3: green (cup)}\\
  \bottomrule
  \end{tabular}
  \caption{An example showing model's ability to estimate objects' depth ordering from a single image.\\Source: photo taken by an author from the ByteDance Seed team.}
  \label{fig:depth_sorting}
\end{figure}

\subsection{Video Temporal Grounding}
\begin{figure}[h]
  \centering
  \begin{tabular}{m{16cm}}
  \toprule
  \begin{center}
  {\small Input video}
  \end{center}
  \begin{center}
  \includegraphics[width=15cm]{figures/videogrounding.pdf}
  \end{center}
  {
  \textbf{Prompt:} Please watch this video and find out all key events in this video, and output the events along with the start/end timestamps.\newline
  \textbf{Model response:} 0.0--3.21 seconds, a girl in a yellow track suit stands on a track, preparing for a run. 3.32--10.02 seconds, she runs down the track, and jumps over a pole, landing on a mat. 10.13--12.16 seconds, she gets up off the mat, and walks away. 12.27--22.36 seconds, a replay of her run and jump is shown.\newline\newline
  \textbf{Prompt:} When does the woman jump? Please output the exact timestamps. If the woman jumps several times, please output the timestamps respectively.\newline
  \textbf{Model response:} 6--8 seconds, 16--22 seconds.
  }\\
  \bottomrule
  \end{tabular}
  \caption{The first query shows the model's ability to summarize/segment key events in a video (\eg, dense video captioning), and the second query shows model's ability of localizing an event in a video (\eg, video grounding).}
  \label{fig:video_grounding_example}
\end{figure}
% \textbf{Prompt:}
% \begin{framed}
% \begin{small}
% \begin{Verbatim}[breaklines=true,breaksymbol=]

% \end{Verbatim}
% \end{small}
% \end{framed}
% \textbf
% \begin{framed}
% \begin{small}
% \begin{Verbatim}[breaklines=true,breaksymbol=]
% 0.0 - 3.21 seconds, a girl in a yellow track suit stands on a track, preparing for a run. 3.32 - 10.02 seconds, she runs down the track, and jumps over a pole, landing on a mat. 10.13 - 12.16 seconds, she gets up off the mat, and walks away. 12.27 - 22.36 seconds, a replay of her run and jump is shown.
% \end{Verbatim}
% \end{small}
% \end{framed}

% \textbf{Prompt:}
% \begin{framed}
% \begin{small}
% \begin{Verbatim}[breaklines=true,breaksymbol=]
% When does the woman jump? Please output the exact timestamps. If the woman jumps several times, please output the timestamps respectively.
% \end{Verbatim}
% \end{small}
% \end{framed}
% \textbf{Model response:}
% \begin{framed}
% \begin{small}
% \begin{Verbatim}[breaklines=true,breaksymbol=]
% 6 - 8 seconds, 16 - 22 seconds.
% \end{Verbatim}
% \end{small}
% \end{framed}
% Source: ActivityNet v1.3.
\clearpage
\subsection{OCR Parsing and Document Understanding}

\begin{figure}[h]
  \centering
  \begin{tabular}{m{6cm}m{10cm}}
  \toprule
  \includegraphics[width=6cm]{figures/doubao_draft.jpg} & 
  {\textbf{Prompts:} Based on the paper, what framework does the author use to achieve fault tolerance?\par \textbf{Model Responses:} According to the paper, to handle various hardware and software faults during the training, the author uses the robust training framework of MegaScale to achieve fault tolerance.\newline\newline
  \textbf{Prompts:} Based on the paper, which one takes longer to train, RL phase or reward model?\par \textbf{Model Responses:}
  \begin{enumerate}
      \item First, find the relevant information in the paper:
      \begin{itemize}
          \item The paper states: ``The RL phase of Seed1.5-VL costs 60k GPU hours. The reward model is trained using the same framework as Seed1.5-VL pretraining phase, requiring 24k GPU hours.''
      \end{itemize}
      \item Then, compare the GPU-hour requirements:
      \begin{itemize}
          \item The RL phase requires 60k GPU hours, and the reward model requires 24k GPU hours.
      \end{itemize}
  \end{enumerate}
  So, the RL phase takes longer to train.\newline\newline
  \textbf{Prompts:} Can you repeat section 5.1.4 but skip the first sentence?\newline
  \textbf{Model Responses:} Once the robust training framework detects a fault, it will trigger the recovery process and recover the training from the last successful checkpoint. We leverage ByteCheckpoint [155] for efficient checkpoint saving and resuming.
  }\\
  \bottomrule
  \end{tabular}
\caption{
Demonstration of \doubao{}'s ability of accurately extracting texts from an image, understanding the user's query, and retrieving the answer from the document. The final example also highlights model's instruction following capability (\eg, ``skip the first sentence'').
\\
Source: a printout of an earlier draft of the technical report.
}
\label{fig:ocr_parse_qa}
\end{figure}

\clearpage

\subsection{Multilingual OCR Parsing}

\begin{figure}[h]
  \centering
  \begin{tabular}{m{6cm}m{10cm}}
  \toprule
  \includegraphics[width=6cm]{figures/long_receipt.jpg} & 
  {\footnotesize {\bf Prompts:} can you extract the dish names, quantities, and their prices into a markdown table?
  \par {\bf Model Responses:}
  \par
  \begin{CJK*}{UTF8}{gbsn}
  \begin{Verbatim}[breaklines=true,breaksymbol=]
| Dish Name | Quantity | Price |
| --- | --- | --- |
| Black Belly (黑毛肚) | 2 | $39.96 |
| Supreme Lamb Shoulder (精选羊肩肉) | 2 | $23.96 |
| Egg Dumplings (蛋饺) | 1 | $8.98 |
| Bean Curd Sheet (干煎豆皮) | 1 | $5.98 |
| Supreme Kobe Beef (极品和牛) | 2 | $59.96 |
| Black Tofu (手工黑豆腐) | 1 | $7.98 |
| Mushroom Platter (菌类拼盘(金针菇,杏鲍菇,香菇)) | 1 | $8.98 |
| Beef Stomach (极品鲜毛肚) | 1 | $11.98 |
| Two Flavour Soup Base (龙门湾鸳鸯锅) | 1 | $15.98 |
| Self Service Sauce Bar (自助调料小吃) | 7 | $20.86 |
| Supreme Goose Intestine (极品鹅肠) | 1 | $22.98 |
| Bamboo Prawn Shrimp Paste (竹荪虾滑) | 1 | $13.98 |
| Shrimp Paste (虾滑) | 1 | $11.98 |
| Quail Egg (鹌鹑蛋) | 1 | $7.98 |
| Spinach (菠菜) | 1 | $4.98 |
| Tongho (茼蒿) | 1 | $5.98 |
| Fried Bean Curd Skin (响铃卷) | 1 | $5.98 |
| Beef Balls (Q弹牛肉丸) | 1 | $7.98 |
| Supreme Fatty Beef (精品肥牛) | 1 | $10.98 |
| Marbled Beef (雪花牛肉) | 1 | $13.98 |
| Beef Short Rib (安格斯牛小排) | 2 | $29.96 |
| Prime Rib Eye Beef (极品肋眼肉) | 1 | $16.98 |
| nine specialties platter (龙门湾至尊九宫格) | 1 | $39.98 |
| Beef Tripe (牛百叶) | 2 | $15.96 |
| House Beef Throat (牛黄喉) | 1 | $11.98 |
\end{Verbatim}
\end{CJK*}
  } \\
  \bottomrule
  \end{tabular}
\caption{An example of extracting multilingual texts from a long receipt.\\
Source: photo taken by an author from the ByteDance Seed team.}
\label{fig:long_receipt}
\end{figure}

\clearpage
\subsection{Generate Code for a Diagram of Novel Format}

\begin{figure}[!h]
  \centering
  \begin{tabular}{m{16cm}}
  \toprule
  \begin{center}
  \includegraphics[width=10cm]{figures/NCAA-Tournament-Printable-Bracket-2025.jpg}
  \end{center}
  {\scriptsize {\bf Prompts:} can you generate the Mermaid code that produce the bracket for ONLY the South region?
  \par {\bf Model Responses:} \texttt{<think>...</think>}Here’s the Mermaid code for the South Region bracket:
  \par
  \begin{Verbatim}[breaklines=true,breaksymbol=]
flowchart TD
    S1[1\nAuburn] --> S1_16[1v16\nAuburn vs Alabama St/St Francis PA]
    S16[16\nAlabama St/St Francis PA] --> S1_16
    S8[8\nLouisville] --> S8_9[8v9\nLouisville vs Creighton]
    S9[9\nCreighton] --> S8_9
    S5[5\nMichigan] --> S5_12[5v12\nMichigan vs UCSD]
    S12[12\nUCSD] --> S5_12
    S4[4\nTexas A&M] --> S4_13[4v13\nTexas A&M vs Yale]
    S13[13\nYale] --> S4_13
    S6[6\nMississippi] --> S6_11[6v11\nMississippi vs San Diego St/UNC]
    S11[11\nSan Diego St/UNC] --> S6_11
    S3[3\nIowa St] --> S3_14[3v14\nIowa St vs Lipscomb]
    S14[14\nLipscomb] --> S3_14
    S7[7\nMarquette] --> S7_10[7v10\nMarquette vs New Mexico]
    S10[10\nNew Mexico] --> S7_10
    S2[2\nMichigan St] --> S2_15[2v15\nMichigan St vs Bryant]
    S15[15\nBryant] --> S2_15
    
    S1_16 --> S2nd1[2nd Round\nWinner 1v16 vs 8v9]
    S8_9 --> S2nd1
    S5_12 --> S2nd2[2nd Round\nWinner 5v12 vs 4v13]
    S4_13 --> S2nd2
    S6_11 --> S2nd3[2nd Round\nWinner 6v11 vs 3v14]
    S3_14 --> S2nd3
    S7_10 --> S2nd4[2nd Round\nWinner 7v10 vs 2v15]
    S2_15 --> S2nd4
    
    S2nd1 --> S3rd1[Elite 8\nWinner 2nd1 vs 2nd2]
    S2nd2 --> S3rd1
    S2nd3 --> S3rd2[Elite 8\nWinner 2nd3 vs 2nd4]
    S2nd4 --> S3rd2
    
    S3rd1 --> SWinner[South Winner\nWinner 3rd1 vs 3rd2]
    S3rd2 --> SWinner
\end{Verbatim}
  }\\
  \bottomrule
  \end{tabular}
\caption{An example of model's several capabilities, such as OCR, coding, instruction following, working together to generate Mermaid code for a portion of the diagram. Summarization texts are omitted from the response. Paste the code into the \href{https://mermaid-js.github.io/mermaid-live-editor/}{Mermaid Live Editor} to visualize the South region bracket.}
\label{fig:ncaa_bracket}
\end{figure}
\clearpage
\subsection{Image-conditioned Creative Writing}

\begin{figure}[h]
  \centering
  \begin{tabular}{m{6cm}m{10cm}}
  \toprule
  \includegraphics[width=6cm]{figures/rings.jpg} & 
  {\textbf{Prompts:} write a romantic poem in English inspired by this picture.
\par
  \textbf{Model Responses:} \texttt{<think>...</think>}
  \par
  \begin{Verbatim}[breaklines=true,breaksymbol=]
Fingers Entwined
  
Beneath the hum of a world that rushes by,
Our hands meet---soft, a silent lullaby.
Your palm, a map of stories yet untold,
My fingers trace the edges, brave and bold.

Rings gleam, twin sparks in this quiet space,
Promises etched in silver’s tender embrace.
Each line, each crease, a secret only we share---
Time slows, as if love itself holds its breath here.

Remember when our shadows first aligned?
Now skin to skin, no distance left to find.
These hands, they’ll carry dawns and midnight’s hush,
Weave years into a tapestry of "us."

For in this touch, a universe unfolds---
Heartbeats syncing, futures yet to hold.
Two hands, one song, forever intertwined---
A language only love could ever design.

  \end{Verbatim}
  \par
The poem mirrors the intimacy of clasped hands, weaving themes of connection, memory, and enduring commitment, with imagery of touch and time to echo the quiet romance in the photograph.
  } \\
  \bottomrule
  \end{tabular}
\caption{An example of image-conditioned creative text generation. The model processes an input image and generates a poem semantically related to the visual content.\\
Source: picture taken by an author from the ByteDance Seed team.}
\label{fig:creative_writing}
\end{figure}

\clearpage

\subsection{Failure Cases: 3D Spatial Imagination}

\begin{figure}[h]
  \centering
  \begin{tabular}{m{6cm}m{10cm}}
  \toprule
  \includegraphics[width=6cm]{figures/rolling_dice.png} & 
  {\textbf{Prompts:} if we move the dice along the arrow directions, what will be the number on top?\par \textbf{Model Responses:} \texttt{<think>...</think>}To determine the number on top after moving the dice along the arrow directions, we analyze the initial configuration and movements:
  \begin{enumerate}
  \item \textbf{Initial Dice Faces}:
    \begin{itemize}
        \item Front: 1 dot (opposite back: 6 dots, $1 + 6 = 7$).
        \item Right: 2 dots (opposite left: 5 dots, $2 + 5 = 7$).
        \item Top: 5 dots (opposite bottom: 2 dots, $5 + 2 = 7$).
    \end{itemize}
  \item \textbf{Movements}:
    \begin{itemize}
        \item \textbf{Down Arrow}: Rolling the die downward (front to bottom) does not affect the top face directly (since top/bottom and front/back are separate axes).
        \item \textbf{Right Arrow}: Rolling the die rightward (right to front) also does not change the top face (top remains independent of right/left movements in this sequence).
    \end{itemize}
  \end{enumerate}
  Thus, the top face (initially 5 dots) remains unchanged after the specified movements.
  \par
  \textbf{Answer}: 5
  }
  \\
  \hline
  \includegraphics[width=6cm]{figures/side_view_projection.png} &
  {\textbf{Prompts:} View the blocks on the left from the orange point and direction of the arrow. Which image on the right is the correct view?
\par \textbf{Model Responses:} \texttt{<think>...</think>}To determine the correct front view from the orange point and arrow direction, analyze the vertical height of each column in the 3D structure:
\begin{itemize}
    \item \textbf{Leftmost column}: 1 cube (bottom layer only).
    \item \textbf{Second column}: 2 cubes (two layers).
    \item \textbf{Third column (central, tallest)}: 3 cubes (three layers).
    \item \textbf{Fourth column}: 2 cubes (two layers).
\end{itemize}
Matching this height distribution (1, 2, 3, 2) to the options:
\begin{itemize}
    \item \textbf{A}: Incorrect (leftmost column too tall).
    \item \textbf{B}: Incorrect (symmetric, not matching the structure).
    \item \textbf{C}: Incorrect (heights don’t align).
    \item \textbf{D}: Correct (heights 1, 2, 3, 2 match the front view).
\end{itemize}
\par
\textbf{Answer:} D
} \\
  \bottomrule
  \end{tabular}
\caption{Two examples where \doubao{}, Gemini 2.5 Pro, and OpenAI o4-mini all failed to produce the correct reasoning. In the \doubao{} case, the reasoning is incorrect despite a correct final answer. This highlights a limitation of contemporary VLMs in tasks requiring robust 3D spatial reasoning.}
\label{fig:failure_spatial_imagination}
\end{figure}

\clearpage

\subsection{Failure Cases: Hallucination (Knowledge Prior)}

\begin{figure}[h]
  \centering
  \begin{tabular}{m{6cm}m{10cm}}
  \toprule
  \includegraphics[width=6cm]{figures/wrong_residual.jpg} & 
  {\footnotesize \textbf{Prompts:} can you generate the DOT code that renders a similar graph to this one?
\par
  \textbf{Model Responses:} \texttt{<think>...</think>}Here's the DOT code to render a graph similar to your Transformer layer diagram:
  \par
  \begin{Verbatim}[breaklines=true,breaksymbol=]
  digraph TransformerLayer {
    rankdir=TB;
    node [fontname="Sans-Serif"];
    
    // Define nodes
    input [label="x_l", shape=rectangle];
    ln1 [label="LN", shape=rectangle];
    mha [label="MHA", shape=rectangle];
    add1 [label="+", shape=circle];
    ln2 [label="LN", shape=rectangle];
    ffn [label="FFN", shape=rectangle];
    add2 [label="+", shape=circle];
    output [label="x_{l+1}", shape=rectangle];
    
    // Define edges
    input -> ln1;
    ln1 -> mha;
    mha -> add1;
    input -> add1;  // Residual connection (first skip)
    
    add1 -> ln2;
    ln2 -> ffn;
    ffn -> add2;
    add1 -> add2;  // Residual connection (second skip)
    
    add2 -> output;
    
    // Optional styling (you can adjust colors/shapes)
    edge [arrowhead="vee", arrowsize=0.8];
    node [style=filled, fillcolor=white, penwidth=1];
    add1, add2 [fillcolor=lightblue];
  }
  \end{Verbatim}
  \par
  $\dots$
  } \\
  \bottomrule
  \end{tabular}
\caption{A case study illustrating the inability of \doubao{}, Gemini 2.5 Pro, and OpenAI o4-mini to generate faithful DOT code when presented with a non-standard FFN residual connection. The drawing shows the network structure, specifically the atypical residual path. All models exhibited a tendency to generate DOT code corresponding to a standard residual connection.}
\label{fig:hallucination}
\end{figure}

\clearpage

\subsection{Failure Cases: Combinatorial Search I}

\begin{figure}[h]
  \centering
  \begin{tabular}{m{16cm}}
  \toprule
  \begin{center}
  Input image
  \end{center}
  \begin{center}
  \includegraphics[width=8cm]{figures/circle_puzzle.png}
  \end{center}
  \\
  {\footnotesize \textbf{Prompts:} In this puzzle, each circle is a prime number (2, 3, 5 or 7), solve puzzle \#6 which only has one solution.\newline\newline
  \textbf{Model Responses:} \texttt{<think>...</think>}
  To solve Puzzle \#6 where each circle represents a prime number (2, 3, 5, or 7), we analyze the multiplication:
  \begin{enumerate}
      \item {\bf Prime Digit Constraints}\newline
      Each digit in the multiplicand (three-digit number), multiplier (two-digit number), and the product must be among 2, 3, 5, or 7. We start by looking at the units place of the multiplication. When we multiply the units digit of the three-digit number and the units digit of the two - digit number, the result's units digit must also be a prime number. Through testing different combinations, we find that the units digit of the three-digit number and the units digit of the two-digit number are likely 5 and 7 (or vice - versa) because $5\times 7=35$, and the units digit 5 is a prime number.
      \item {\bf Testing Combinations}\newline
      We try out different three-digit and two-digit numbers composed of prime digits. After a series of trials, we consider the three-digit number 325 and the two-digit number 77.
      \begin{itemize}
          \item[--] First, calculate $325 \times7 = 2275$. Here, each digit 2, 2, 7, and 5 is a prime number.
          \item[--] Then, calculate $325 \times 70=22750$. Although there is a 0 in this result, which seems to be a problem as 0 is not a prime number, we need to look at the overall structure of the. When we add  and  in the, we get 25025.
      \end{itemize}
      \item {\bf Conclusion}\newline
      Even though there is a 0 in the intermediate step, this is the only combination that comes close to satisfying the prime-digit rule for the majority of the digits. Given the constraints of the puzzle, we can conclude that the solution is based on the multiplication $325 \times 77=25025$.
  \end{enumerate}
  {\bf Final Answer}\newline
  The solution, considering the prime-digit pattern and the structure of the multiplication, is represented by the digits in the multiplication process, and the key combination is $\mathbf{325 \times 77}$, with the understanding of the prime-digit constraints in the puzzle.}
  \\
  \bottomrule
  \end{tabular}
\caption{A case study revealing limitations of \doubao{}, Gemini 2.5 Pro, and OpenAI o4-mini on a puzzle requiring combinatorial search. The puzzle involves determining a two-digit and a three-digit number, where each digit must be a prime number from the set $\{2, 3, 5, 7\}$. The size of the search space ($4^5=1024$ combinations) appears to exceed the current capabilities of these models for reliable reasoning.}
\label{fig:brute_force_search}
\end{figure}

\clearpage

\subsection{Failure Cases: Combinatorial Search II}

\begin{figure}[h]
  \centering
  \begin{tabular}{m{16cm}}
  \toprule
  \begin{center}
  Input image
  \end{center}
  \begin{center}
  \includegraphics[width=8cm]{figures/counting_squares.png}
  \end{center}
  \\
  {\textbf{Prompts:} count the number of squares in the image including the ones made of multiple smaller squares.\newline\newline
  \textbf{Model Responses:} \texttt{<think>...</think>}\newline
  To count all squares (including those formed by smaller squares), we identify squares of different sizes:
  \begin{itemize}
      \item $\mathbf{1\times 1}: 10$
      \item $\mathbf{2\times 2}: 4$
      \item $\mathbf{3\times 3}: 2$
      \item $\mathbf{4\times 4}: 1$
  \end{itemize}
  Summing these: $10 + 4 + 2 + 1=17$.\newline
  {\bf Answer: 17}}
  \\
  \bottomrule
  \end{tabular}
\caption{Example demonstrating the inability of \doubao{}, Gemini 2.5 Pro, and OpenAI o4-mini to correctly count all squares within the image. This performance indicates a challenge for existing VLMs in performing exhaustive visual enumeration or recognizing complex arrangements of simple shapes.}
\label{fig:brute_force_search2}
\end{figure}

\clearpage

\section{Evaluation Details}
\label{app:eval_detail}
\subsection{Internal Benchmark Structure}
\label{sec:app:internal_benchmark}
Our internal benchmark is structured as a hierarchical tree, as illustrated in \cref{tab:eval_taxonomy}. The top level comprises two nodes: vision capability and integrated capability. This structure is further subdivided into 11 level-2, 43 level-3, and 29 level-4 categories, with each successively deeper level representing increasingly fine-grained capabilities.

This fine-grained categorization proves critical during our model development process. It allows us to precisely identify specific capabilities that may be deficient in the current iteration, gauge the improvements achieved over previous iterations, and inform future development efforts by guiding the focus towards areas requiring further enhancement.

\begingroup

\scriptsize
\begin{longtable}{|l|l|l|l|r|}
\caption{Structure of the internal evaluation benchmark, categorized by capability level. Includes accuracy metrics for each capability, defined as the alignment rate between LLM-as-a-judge assessments and human evaluations. Table continued on next page.}
\label{tab:eval_taxonomy}\\
\hline
{\bf \makecell[l]{Level-1\\Capabilities}} & {\bf \makecell[l]{Level-2\\Capabilities}} & {\bf \makecell[l]{Level-3\\Capabilities}} & {\bf \makecell[l]{Level-4\\Capabilities}} & {\bf Accuracy} \\
\hline
\multirow{32}{*}{\makecell[l]{Vision\\Capabilities}} & \multirow{7}{*}{Perception} & Status & & 93.3\% \\
& & Count & & 99.3\% \\
& & Find The Difference & & 95.3\% \\
& & Spatial Understanding & & 100.0\% \\
& & Property & & 98.7\% \\
& & Activity & & 95.3\% \\
& & Visual Prompt & & 97.3\% \\
\cline{2-5}
& \multirow{12}{*}{Recognition} & Commodity & & 93.3\% \\
& & Arts & & 97.3\% \\
& & Museum & & 95.3\% \\
& & Engineering & & 99.3\% \\
& & Face & & 99.3\% \\
& & Nature & & 96.7\% \\
& & Health \& Medicine & & 99.3\% \\
& & Entertainment & & 100.0\% \\
& & Landmark & & 100.0\% \\
& & Animals \& Plants & & 93.3\% \\
& & Food & & 95.3\% \\
\cline{2-5}
& \multirow{8}{*}{OCR} & \multirow{8}{*}{OCR QA} & Flowchart & 98.7\% \\
& & & Table & 100.0\% \\
& & & Scene Text & 99.3\% \\
& & & Mix & 100.0\% \\
& & & Doc & 100.0\% \\
& & & chart & 96.0\% \\
& & & Formula & 100.0\% \\
& & & Other & 100.0\% \\
\cline{2-5}
& \multirow{2}{*}{\makecell[l]{Caption \&\\Counterfactual}} & \multirow{2}{*}{Counterfactual} & Unanswerable & 94.7\% \\
& & & Prompt Image Mismatch & 96.0\% \\
\hline
\pagebreak
\hline
\multirow{39}{*}{\makecell[l]{Integrated\\Capabilities}} & \multirow{4}{*}{Reasoning} & Visual Puzzle & & 100.0\% \\
& & Event Forecasting & & 99.3\% \\
& & ARC-AGI Vision (in-house) & & 100.0\% \\
& & Planning & & 98.0\% \\
\cline{2-5}
& \multirow{4}{*}{\makecell[l]{Document \& Diagram\\Understanding}} & Summarization & & 91.3\% \\
\cline{3-3}
& & \makecell[l]{Reasoning over Document/Diagram\\and Open Knowledge} & & 98.0\% \\
\cline{3-5}
& & \multirow{2}{*}{Translation} & Minor Languages Translation & 93.8\% \\
& & & Translation between Chinese and English & 87.3\% \\
\cline{2-5}
& \multirow{4}{*}{Agent} & \multirow{2}{*}{GUI Agent} & Mobile \& Computer Screen Understanding & 96.2\% \\
& & & multi step GUI Reasoning & 96.0\% \\
\cline{3-5}
& & Embodied Agent & & 99.3\% \\
& & VLN \& Autonomous Driving & & 99.3\% \\
\cline{2-5}
& \multirow{4}{*}{\makecell[l]{Atomic Instruction\\Following}} & \multirow{3}{*}{Text Atomic instruction} & Output Format & 75.4\% \\
& & & Conditional Rules & 87.3\% \\
& & & Forbid & 90.7\% \\
\cline{3-5}
& & Visual Atomic instruction & & 100.0\% \\
\cline{2-5}
& \multirow{3}{*}{To B} & Categorization & & 97.9\% \\
\cline{3-3}
& & \makecell[l]{Reasoning over Document/Diagram\\and Open Knowledge} & & 96.7\% \\
\cline{3-3}
& & Structured Information Extraction & & 93.3\% \\
\cline{2-5}
& \multirow{15}{*}{OOD} & \multirow{3}{*}{Spatial \& Temporal Understanding} & Indoor Directional Reasoning & 100.0\% \\
& & & Satellite Image Matching & 99.3\% \\
& & & Scene View Sorting & 97.3\% \\
\cline{3-5}
& & Multi-turn Multi-image Reasoning & & 100.0\% \\
\cline{3-5}
& & \multirow{2}{*}{Perception Hard} & Indoor Deduplication Counting & 98.0\% \\
& & & Same Room Detection & 97.3\% \\
\cline{3-5}
& & Judgment and Reflection & & 72.7\% \\
& & Other & & 100.0\% \\
\cline{3-5}
& & \multirow{7}{*}{Visual Puzzle} & Puzzles and Games & 100.0\% \\
& & & Jigsaw Puzzle & 97.3\% \\
& & & Comic Ordering & 100.0\% \\
& & & Unblock Me & 97.3\% \\
& & & Chess & 100.0\% \\
& & & Maze L6 & 99.3\% \\
& & & Maze L10 & 100.0\% \\
\cline{2-5}
& \multirow{3}{*}{Knowledge} & World Knowledge & & 100.0\% \\
& & College-level subject knowledge & & 100.0\% \\
& & K12 & & 100.0\% \\
\hline
\end{longtable}
\endgroup
\clearpage

\subsection{Comprehensive Comparisons on internal benchmarks}
\label{sec:app:complete_comparison}
\Cref{fig:internal_complete_comparison} presents a comprehensive comparison of \doubao{} with eight prominent model families: Gemini, GPT, Claude, Qwen, Llama, InternVL, StepFun, and GLM. Overall, \doubao{} ranks second. Grouping models strictly by parameter count proves challenging as specific parameter details are not publicly disclosed for many models. Our model's size is comparable to Llama 4 Maverick, which is reported to utilize 17 billion active parameters and employs a Mixture-of-Experts (MoE) architecture. Our evaluation demonstrates that \doubao{} achieves significantly better performance than Llama 4 Maverick on this benchmark. For certain model families, we include different model releases to assess the progress within the community over time. Our evaluation highlights that \textit{thinking} models dominate the top-5 ranking, which we attribute to the internal benchmark's focus on measuring integrated model capabilities. Consistent with community trends, newer model releases from the same provider generally outperform earlier iterations; for example, GPT-4o-Latest achieves higher scores than GPT-4o-0513, and Gemini 2.5 surpasses Gemini 2.0.
\begin{figure}[ht]
\centering
\includegraphics[width=0.9\textwidth]{figures/internal_complete_comparison.pdf}
\caption{A comprehensive comparison of the \doubao{} model against existing models, ordered according to their overall performance on our internal benchmark. Models employing a \textit{thinking} methodology are delineated by red bars, whereas those classified as \textit{non-thinking} are represented by blue bars. Analysis of the top-5 scores reveals a predominance of \textit{thinking} models. To account for potential updates to model APIs, the API release date (in the format of year-month-day) is appended to each model name.}
\label{fig:internal_complete_comparison}
\end{figure}
\clearpage
\subsection{Capabilities and Benchmark Tasks}
\label{sec:benchmarks}
We use 60 public benchmarks to evaluate \doubao{} across ten different capabilities: multimodal reasoning, general visual question answering, document and chart understanding, visual grounding and counting, spatial understanding, short and long video understanding, streaming video understanding, video grounding, GUI agent. Below, we provide a detailed list of all benchmarks.
\begin{itemize}
\item \textbf{Multimodal Reasoning:} We use seven benchmarks: MMMU~\cite{yue2024mmmu}, MMMU-Pro~\cite{yue2024mmmupro}, MathVision~\cite{wang2024measuring}, OlympiadBench~\cite{he2024olympiadbench}, MathVista~\cite{lu2023mathvista}, V\textsuperscript{*}~\cite{wu2023vguidedvisualsearch}, VLM are Blind~\cite{rahmanzadehgervi2025visionlanguagemodelsblind}, ZeroBench~(Main/Subtasks)~\cite{roberts2025zerobenchimpossiblevisualbenchmark}, 
VisuLogic~\cite{xu2025visulogicbenchmarkevaluatingvisual},
Video-MMMU~\cite{hu2025video}, and MMVU~\cite{zhao2025mmvu}.
\item \textbf{General Visual Question Answering:} We use eight benchmarks: RealWorldQA~\cite{realworldqa2024}, MMStar~\cite{chen2024we}, MMVet~\cite{yu2023mm}, MMBench (English and Chinese)~\cite{liu2024mmbench}, MMVP~\cite{tong2024eyes}, HallusionBench~\cite{guan2024hallusionbench}, and BLINK~\cite{fu2024blink}.
\item \textbf{Document and Chart Understanding:} We use seven benchmarks: TextVQA~\cite{singh2019towards}, AI2D~\cite{kembhavi2016diagram}, ChartQA~\cite{masry2022chartqa}, InfographicVQA~\cite{mathew2022infographicvqa}, DocVQA~\cite{mathew2021docvqa}, OCRBench~\cite{liu2024ocrbench}, and CharXiv~(RQ/DQ)~\cite{wang2024charxiv}.
\item \textbf{Grounding and Counting:} We use five benchmarks: LVIS-MG (multi-object grounding derived from LVIS~\cite{gupta2019lvis}), VisualWebBench~\cite{liu2024visualwebbench}, RefCOCO~\cite{refcoco,refcocog,referit}, CountBench~\cite{paiss2023teaching}, FSC-147~\cite{ranjan2021learning}.
\item \textbf{Spatial Understanding:} We use five benchmarks: DA-2K~\cite{depth_anything_v2}, NYU-Depth V2~\cite{Silberman2012indoor}, SUN-RGBD~\cite{song2015sun}, ARKitScenes~\cite{baruch2021arkitscenes}, and All-Angles Bench~\cite{yeh2025seeing}.
\item \textbf{Short Video Understanding:} We use six benchmarks: MotionBench~\cite{hong2025motionbench}, MVBench~\cite{li2024mvbench}, TOMATO~\cite{shangguan2024tomato}, TVBench~\cite{cores2024tvbench}, Dream-1K~\cite{wang2024tarsierrecipestrainingevaluating}, and TempCompass~\cite{liu2024tempcompass}.
\item \textbf{Long Video Understanding:} We use six benchmarks: LongVideoBench~\cite{wu2024longvideobench}, LVBench~\cite{wang2024lvbench}, MLVU~\cite{zhou2024mlvu}, VideoMME~\cite{fu2024video}, TemporalBench~\cite{cai2024temporalbench}, and EgoSchema~\cite{mangalam2023egoschema}.
\item \textbf{Streaming Video Understanding:} We use six benchmarks: OVBench~\cite{ovbench}, OVOBench~\cite{li2025ovo}, StreamBench~\cite{xiong2025streaming}, and StreamingBench~\cite{lin2024streamingbench}.
\item \textbf{Video Grounding:} We use two benchmarks: Charades-STA~\cite{gao2017tall} and TACoS~\cite{gao2017tall}.
\item \textbf{GUI Agent:} We use seven benchmarks: ScreenSpot-V2~\cite{wu2024atlas}, ScreenSpot-Pro~\cite{li2025screenspot}, OSWorld~\cite{xie2024osworld}, Windows Agent Arena~\cite{bonatti2024windows}, WebVoyager~\cite{he2024webvoyager}, Online-Mind2Web~\cite{xue2025illusion}, and Android World~\cite{rawles2024androidworld}.
\end{itemize}

\clearpage
\subsection{Evaluation Prompts}
All benchmarks are evaluated 0-shot using an instruction-tuned model.
To activate thinking mode of \doubao{}, we add the following preamble:
\begin{framed}
\begin{Verbatim}[breaklines=true,breaksymbol=]
You should first think about the reasoning process in the mind and then provide the user with the answer. The reasoning process is enclosed within <think> </think> tags, i.e. <think> reasoning process here </think> answer here
\end{Verbatim}
\end{framed}
Then, we follow it with a prompt that is customized for each benchmark. Prompt templates for each benchmark are listed below. 
In each template, \texttt{\{question\}} is filled with the actual sample's question, \texttt{\{options\}} is replaced with sample's multiple-choice answer options, \texttt{<image>} is filled with computed ViT embeddings of the input image, \texttt{<label>} is replaced with the object's label (\eg, grounding benchmarks), and \texttt{<video>} is filled with the ViT embeddings of the video frames (\eg, video benchmarks). Below, we omit the \texttt{[SOI]} and \texttt{[EOI]} tokens wrapped around each image.

\paragraph{MMMU}
We use the same metric suggested by OpenCompass~\footnote{\url{https://github.com/open-compass/opencompass}}. We follow the same image position placeholder as the original samples in MMMU, which can be interleaved.
\begin{framed}
\begin{Verbatim}[breaklines=true,breaksymbol=]
<image>
Question: {question}
Options:
{options}
Your response can be freely expressed in any format, but the final answer must be presented in this format:
"Final answer: [the correct option]"
\end{Verbatim}
\end{framed}

\paragraph{MMMU-Pro}
We use official metric of MMMU-Pro.
\begin{framed}
\begin{Verbatim}
<image>
{question}
\end{Verbatim}
\end{framed}

\paragraph{MathVision}
As suggested by \citet{wang2024measuring}, curation of prompt engineering is essential for objective and precise evaluation on MathVision.
We use official metric of MathVision.
We notice thinking models, such as OpenAI-O1, sometimes provide solutions that cannot be precisely parsed by the official rule-based verifier provided by MathVision, \eg, prediction 2kg v.s. groundtruth 2, or providing value of the correct option instead of the name of option.
Therefore, we carefully design the prompt for OpenAI-O1 to avoid potential underestimation. And we use the same prompt to test \doubao{} and Gemini-2.5-Pro on this benchmark.
\begin{framed}
\begin{Verbatim}[breaklines=true,breaksymbol=]
<image>
{question}
Please solve the problem step by step and put your answer in one "\boxed{}". If it is a multiple choice question, only one letter ("\boxed{A}", "\boxed{B}", "\boxed{C}", "\boxed{D}", or "\boxed{E}") is allowed in the "\boxed{}". For example, do NOT output "\boxed{42}" for a multiple choice question.
\end{Verbatim}
\end{framed}

\paragraph{OlympiadBench}
We use official metric of OlympiadBench.
\begin{framed}
\begin{Verbatim}
<image>
{question}
\end{Verbatim}
\end{framed}

\paragraph{MathVista}
We use the same metric suggested by OpenCompass.
\begin{framed}
\begin{Verbatim}
<image>
{question}
\end{Verbatim}
\end{framed}

\paragraph{V*}
We use official metric of V*.
\begin{framed}
\begin{Verbatim}
<image>
{question}
\end{Verbatim}
\end{framed}

\paragraph{VLM are Blind}
We use official metric of VLM are Blind.
\begin{framed}
\begin{Verbatim}
<image>
{question}
\end{Verbatim}
\end{framed}

\paragraph{TextVQA}
We use the same metric suggested by OpenCompass.
\begin{framed}
\begin{Verbatim}
<image>
{question}
Answer the question using a single word or phrase.
\end{Verbatim}
\end{framed}

\paragraph{AI2D}
We use the same metric suggested by OpenCompass.
\begin{framed}
\begin{Verbatim}
<image>
Question: {question}
Options:
{}
Please select the correct answer from the options above.
\end{Verbatim}
\end{framed}

\paragraph{ChartQA}
We use the official metric of ChartQA. The correctness tolerates certain error ratio defined by max\_relative\_change.
\begin{framed}
\begin{verbatim}
<image>
{question}
Answer the question using a single word or phrase.
\end{verbatim}
\end{framed}

\paragraph{InfographicVQA}
We collect scores by uploading prediction to the official leaderboard.
\begin{framed}
\begin{verbatim}
<image>
{question}
Answer the question using a single word or phrase.
\end{verbatim}
\end{framed}

\paragraph{DocVQA}
We collect scores by uploading prediction to the official leaderboard.
\begin{framed}
\begin{verbatim}
<image>
{question}
Answer the question using a single word or phrase.
\end{verbatim}
\end{framed}

\paragraph{OCRBench}
We use the official metric of OCRBench, including lowercase the answers and space removal.
\begin{framed}
\begin{verbatim}
<image>
{question}
\end{verbatim}
\end{framed}

\paragraph{CharXiv}
We use the official metric of Charxiv.
\begin{framed}
\begin{verbatim}
<image>
{question}
\end{verbatim}
\end{framed}

\paragraph{RealWorldQA}
We use the same metric suggested by OpenCompass.
\begin{framed}
\begin{verbatim}
<image>
Question: {question}
Options:
{options}
Please select the correct answer from the options above.
\end{verbatim}
\end{framed}

\paragraph{MMStar}
We use the same metric suggested by OpenCompass.
\begin{framed}
\begin{verbatim}
<image>
Question: {question}
Options:
{options}
Please select the correct answer from the options above.
\end{verbatim}
\end{framed}

\paragraph{MMBench-en}
We use the same metric suggested by OpenCompass.
\begin{framed}
\begin{Verbatim}
<image>
Question: {question}
Options:
{options}
Answer with the option's letter from the given choices directly. The correct option is:
\end{Verbatim}
\end{framed}

\paragraph{MMBench-cn}
We use the same metric suggested by OpenCompass.
\begin{framed}
\begin{CJK*}{UTF8}{gbsn}
\begin{verbatim}
<image>
问题: {question}
选项:
{options}
请根据选项直接回答选项字母。正确选项为：
\end{verbatim}
\end{CJK*}
\end{framed}

\paragraph{MMVP}
We use the official metric of MMVP. This dataset is composed of 150 pairs of samples, each pair containing two questions, considered correct only when both questions are correct.
\begin{framed}
\begin{verbatim}
<image>
{question}
\end{verbatim}
\end{framed}

\paragraph{HallusionBench}
We use the same metric suggested by OpenCompass.
\begin{framed}
\begin{verbatim}
<image>
{question}
\end{verbatim}
\end{framed}

\paragraph{BLINK}
We use the same metric suggested by OpenCompass.
\begin{framed}
\begin{verbatim}
<image>
Question: {question}
Options:
{options}
Please select the correct answer from the options above.
\end{verbatim}
\end{framed}

\paragraph{CountBench}
\begin{framed}
\begin{verbatim}
<image>
{question}
\end{verbatim}
\end{framed}

\paragraph{VisualWebBench}
\begin{framed}
\begin{verbatim}
<image>
{question}
\end{verbatim}
\end{framed}

\paragraph{FSC-147}
\begin{framed}
\begin{Verbatim}[breaklines=true,breaksymbol=]
<image>
Count the number of {label}.\nYou need to point them out first in <point>x y</point> format.
\end{Verbatim}
\end{framed}

\paragraph{LVIS}
\begin{framed}
\begin{Verbatim}[breaklines=true,breaksymbol=]
<image>
Which region does {label} describe? Output the location as <bbox>x1 y1 x2 y2</bbox>.
\end{Verbatim}
\end{framed}

\paragraph{RefCOCO}
\begin{framed}
\begin{Verbatim}[breaklines=true,breaksymbol=]
<image>
which region does text {label} describe? Output the location as <bbox>x1 y1 x2 y2</bbox>.
\end{Verbatim}
\end{framed}

\paragraph{DA-2K}
\begin{framed}
\begin{Verbatim}[breaklines=true,breaksymbol=]
<image>
There are two points with different colors in the image, point1 (denoted with blue point) and point2 (denoted with green point), each representing an object. Which object represented by these points is closer to me? Only provide the answer: 'point1' or 'point2'.
\end{Verbatim}
\end{framed}
\newpage
\paragraph{NYU-Depth V2}
\begin{framed}
\begin{Verbatim}[breaklines=true,breaksymbol=]
<image>
Here are the detailed camera parameters for the image. Camera intrinsic parameters: Focal length f_x={fx}, f_y={fy}. Principal point coordinate locates at the center of the image, c_x={cx} and c_y={cy}, when image width {width} and height {height}. We do not consider distortion parameters here. Therefore, the intrinsic matrix K = [[{fx}, 0, {cx}], [0, {fy}, {cy}], [0, 0, 1]]. Here, we take the camera coordinate system as the world coordinate system and estimate the absolute depth between camera and the object. Estimate the absolute distance between the photographer and object A (marked with a red dot in the image). Respond directly with the absolute distance in meters only.
\end{Verbatim}
\end{framed}

\paragraph{SUN RGB-D}
\begin{framed}
\begin{Verbatim}[breaklines=true,breaksymbol=]
<image>
Here are the detailed camera parameters for the image. Camera intrinsic parameters: Focal length f_x={fx}, f_y={fy}. Principal point coordinate locates near the center of the image, c_x={cx} and c_y={cy}, when image width {width} and height {height}. We do not consider distortion parameters here. Therefore, the intrinsic matrix K = [[{fx}, 0, {cx}], [0, {fy}, {cy}], [0, 0, 1]]. Camera coordinate: X-axis points rightward, Y-axis points downward, and Z-axis points forward. The origin point is the camera location. We take the camera coordinate system as the world coordinate system, namely the camera extrinsic matrix is [[1, 0, 0, 0], [0, 1, 0, 0], [0, 0, 1, 0]]. Please output each 3D bounding box in the following format: <3dbbox>x_center y_center z_center x_size y_size z_size pitch yaw roll</3dbbox>. Note: (1) x_center, y_center, z_center: the center of the object in the camera coordinate, in meters. (2) x_size, y_size, z_size: The dimensions of the object along the XYZ axes, in meters, when the rotation angles are zero. (3) pitch, yaw, roll: Euler angles representing rotations around the X, Y, and Z axes, respectively. Each angle is normalized to the range of (-1, 1) and is multiplied by 180 to convert it into degrees. Detect all {} in this image and display the results in the form of 3D bounding boxes.
\end{Verbatim}
\end{framed}

\paragraph{All-Angles Bench}
\begin{framed}
\begin{Verbatim}[breaklines=true,breaksymbol=]
<image>
Question: {question} Options: {options}. Answer with the option's letter from the given choices directly.
\end{Verbatim}
\end{framed}

\paragraph{OVBench}
\begin{framed}
\begin{verbatim}
<image>
{question} The choices are: [{options}]. The answer is:
\end{verbatim}
\end{framed}

\paragraph{OVOBench}
\begin{framed}
\begin{verbatim}
<image>
{question} The choices are: [{options}]. The answer is:
\end{verbatim}
\end{framed}

\paragraph{StreamingBench{\scriptsize (proactive)}}
\begin{framed}
\begin{Verbatim}[breaklines=true,breaksymbol=]
You will be given an instruction and a video, which requires you to continuosly monitor the video stream and make responses. The instruction is: [{question}]. You are required to determine whether it is the right time to make a response at the end of each frame.
<video>
\end{Verbatim}
\end{framed}

\paragraph{EgoSchema}
\begin{framed}
\begin{Verbatim}[breaklines=true,breaksymbol=]
<video>
You will be given a question about a video and five possible answer options, where C refers to the person wearing the camera. You will be provided frames from the video, sampled evenly across the video. {question} Possible answer choices:{options}
Directly output the final answer in the format "X" where X is the correct letter choice. Never say "unknown" or "unsure", or "None", instead provide your most likely guess.
\end{Verbatim}
\end{framed}

\paragraph{Video-MME}
\begin{framed}
\begin{Verbatim}[breaklines=true,breaksymbol=]
<video>
Select the best answer to the following multiple-choice question based on the video. 
Respond with only the letter (A, B, C, or D) of the correct option.
{question} Possible answer choices:
{options}
The best answer is:
\end{Verbatim}
\end{framed}

\paragraph{TemporalBench}
\begin{framed}
\begin{Verbatim}[breaklines=true,breaksymbol=]
<video>
Select the best answer to the following binary-choice question based on the video. Respond with only the letter (A or B) of the correct option.
{question} Possible answer choices:
{options}
The best answer is:
\end{Verbatim}
\end{framed}

\paragraph{LongVideoBench}
\begin{framed}
\begin{Verbatim}[breaklines=true,breaksymbol=]
<video>
Select the best answer to the following multiple-choice question based on the video. Respond with only the letter of the correct option.
{question} Possible answer choices:
{options}
The best answer is:
\end{Verbatim}
\end{framed}

\paragraph{LVBench}
\begin{framed}
\begin{Verbatim}[breaklines=true,breaksymbol=]
<video>
Select the best answer to the following multiple-choice question based on the video. Respond with only the letter of the correct option.
{question} Possible answer choices:
{options}
The best answer is:
\end{Verbatim}
\end{framed}

\paragraph{MLVU}
\begin{framed}
\begin{Verbatim}[breaklines=true,breaksymbol=]
<video>
Select the best answer to the following multiple-choice question based on the video. Respond with only the letter of the correct option.
{question} Possible answer choices:
{options}
The best answer is:
\end{Verbatim}
\end{framed}

\paragraph{MotionBench}
\begin{framed}
\begin{Verbatim}[breaklines=true,breaksymbol=]
<video>
Select the best answer to the following multiple-choice question based on the video. Respond with only the letter of the correct option.
{question} Possible answer choices:
{options}
The best answer is:
\end{Verbatim}
\end{framed}

\paragraph{MMVU}
\textbf{Open-ended:}
\begin{framed}
\begin{Verbatim}[breaklines=true,breaksymbol=]
<video>
Question: {question}

Answer the given question step by step. Begin by explaining your reasoning process clearly. Conclude by stating the final answer using the following format: 'Therefore, the final answer is: 'Answer: $$ANSWER' (without quotes), where $$ANSWER is the final answer of the question. Think step by step before answering.
\end{Verbatim}
\end{framed}
\textbf{Multiple-choice:}
\begin{framed}
\begin{Verbatim}[breaklines=true,breaksymbol=]
<video>
Question: {question}
Options:
{options}

Answer the given multiple-choice question step by step. Begin by explaining your reasoning process clearly. Conclude by stating the final answer using the following format: 'Therefore, the final answer is: $$LETTER' (without quotes), where $$LETTER is one of the options. Think step by step before answering.
\end{Verbatim}
\end{framed}

\paragraph{Video-MMMU}

1. Open-ended:
\begin{framed}
\begin{Verbatim}[breaklines=true,breaksymbol=]
<video>
Question: {question}

Do not generate any intermediate reasoning process. Directly output the final short answer.
\end{Verbatim}
\end{framed}
2. Multiple-choice:
\begin{framed}
\begin{Verbatim}[breaklines=true,breaksymbol=]
<video>
Select the best answer to the following multiple-choice question based on the video. Respond with only the letter of the correct option.
{question} Possible answer choices:
{options}
The best answer is:
\end{Verbatim}
\end{framed}

\paragraph{MVBench}
\begin{framed}
\begin{Verbatim}[breaklines=true,breaksymbol=]
<video>
Select the best answer to the following multiple-choice question based on the video. Respond with only the letter of the correct option.
{question} Possible answer choices:
{options}
The best answer is:
\end{Verbatim}
\end{framed}

\paragraph{TOMATO}
\begin{framed}
\begin{Verbatim}[breaklines=true,breaksymbol=]
<video>
Select the best answer to the following multiple-choice question based on the video. Respond with only the letter (A, B, C, D, E, F, G, H...) of the correct option.
{question} Possible answer choices:
{options}
The best answer is:
\end{Verbatim}
\end{framed}

\paragraph{TVBench}
\begin{framed}
\begin{Verbatim}[breaklines=true,breaksymbol=]
<video>
Select the best answer to the following multiple-choice question based on the video. Respond with only the letter (A, B, C, D...) of the correct option.
{question} Possible answer choices:
{options}
The best answer is:
\end{Verbatim}
\end{framed}

\paragraph{DREAM-1K}
\begin{framed}
\begin{Verbatim}[breaklines=true,breaksymbol=]
<video>
Describe the video in one paragraph, mainly focusing on the dynamic events in the video. Don’t describe feelings or atmosphere.{question}
\end{Verbatim}
\end{framed}

\paragraph{TempCompass}

1. Multiple-choice QA:
\begin{framed}
\begin{Verbatim}[breaklines=true,breaksymbol=]
<video>
{question} Choices are: {options}
Please directly give the best option:
\end{Verbatim}
\end{framed}

2. Yes/No QA:
\begin{framed}
\begin{Verbatim}[breaklines=true,breaksymbol=]
<video>
{question}
\end{Verbatim}
\end{framed}
3. Caption matching:
\begin{framed}
\begin{Verbatim}[breaklines=true,breaksymbol=]
<video>
{question}
\end{Verbatim}
\end{framed}
4. Caption generation:
\begin{framed}
\begin{Verbatim}[breaklines=true,breaksymbol=]
<video>
{question}
\end{Verbatim}
\end{framed}

\paragraph{Charades-STA}
\begin{framed}
\begin{Verbatim}[breaklines=true,breaksymbol=]
<video>
Find start and end seconds for: "{label}", please return the start and end seconds.
\end{Verbatim}
\end{framed}

\paragraph{TACoS}
\begin{framed}
\begin{Verbatim}[breaklines=true,breaksymbol=]
<video>
Find start and end seconds for: "{label}", please return the start and end seconds.
\end{Verbatim}
\end{framed}
